# Supplementary material for: Computational Reverse Engineering Analysis of Scattering Experiments Method for Interpretation of 2D Small-Angle Scattering Profiles (CREASE-2D)
Source: arXiv:2401.12381 source file (2024-01-22)
Supplement: Supplementary file 1 [file supporting_information.pdf]

# SUPPORTING INFORMATION:
# Computational Reverse Engineering Analysis of Scattering Experiments Method for Interpretation of 2D Small-Angle Scattering Profiles (CREASE-2D)

Sri Vishnuvardhan Reddy Akepati,[1,†] Nitant Gupta,[2,†] and Arthi Jayaraman[2,3,‡]

[1] *Data Science Program, University of Delaware, Newark, DE 19716 USA.*

[2] *Department of Chemical and Biomolecular Engineering, University of Delaware, Newark, DE 19716 USA.*

[3] *Department of Materials Science and Engineering, University of Delaware, Newark, DE 19716 USA.*

## S1. MONTE CARLO SAMPLING OF STRUCTURAL FEATURES IN THE DATASET

Using five uniformly distributed random numbers $(u_1, u_2, ..., u_5)$, each defined between 0 and 1; we can sample five of the six structural features as described below. Only $\phi$ is not sampled, and is instead obtained after the execution of the CASGAP code to generate the structure with a target volume fraction $\phi_{\text{target}} = 0.5$.

### S1.1. Mean and Standard Deviations of the Volumetric Radius ($R_\mu$, $R_\sigma$)

$R_\mu$, $R_\sigma$ are sampled using the first two random numbers $u_1$ and $u_2$. These values are the parameters that will describe the log-normal distribution of the volumetric radius $R$ of all the spheroidal particles in the structure. Accordingly, we can use $r_\mu$ and $r_\sigma$ as analogous parameters that describe a normal distribution, such that:

$$R_\mu = \exp\left(r_\mu + \frac{r_\sigma^2}{2}\right) \tag{1}$$

$$R_\sigma^2 = \exp\left(r_\mu^2 - 1\right)\exp\left(2r_\mu + r_\sigma^2\right) \tag{2}$$

Here, $r_\mu$ is sampled as:

$$r_\mu = \ln(3) + u_1 \ln(10) \tag{3}$$

This equation ensures that at $u_1 = 0$, $r_\mu = r_\mu^{\min}$ is $\ln(3)$ and at $u_1 = 1$, $r_\mu = r_\mu^{\max}$ which is $\ln(30)$, which are the natural logarithms of the two extents of the mean volumetric radius as described in the main text. $r_\sigma$ is sampled using both $u_1$ and $u_2$ as:

$$r_\sigma = (1 - |2u_1 - 1|)\frac{\ln(10)}{6}u_2 \tag{4}$$

The expression for $r_\sigma$ is designed to make it approach zero whenever $u_1 = 0$ or $u_1 = 1$, and becomes its maximum value of $\frac{\ln(10)}{6}u_2$ at $u_1 = 0.5$. The magnitude of the maximum value can only be $\frac{\ln(10)}{6}$ at $u_2 = 1$, which is 1/6th value of $r_\mu^{\max} - r_\mu^{\min}$. Such a value was arrived at from prior experience with structure generation, and to keep the dispersity in size within the $3\sigma$ limit of the normal distribution.

### S1.2. Mean and Standard Deviations of the Aspect Ratio ($\gamma_\mu, \gamma_\sigma$)

$\gamma_\mu$, $\gamma_\sigma$ are sampled using the next two random numbers $u_3$ and $u_4$. These values are the parameters that will describe the log-normal distribution of the aspect ratio $\gamma$ of all the spheroidal particles in the structure. Similar to the previous section, we can use $g_\mu$ and $g_\sigma$ as analogous parameters that describe a normal distribution, such that:

$$\gamma_\mu = \exp\left(g_\mu + \frac{g_\sigma^2}{2}\right) \tag{5}$$

$$\gamma_\sigma^2 = \exp\left(g_\mu^2 - 1\right)\exp\left(2g_\mu + g_\sigma^2\right) \tag{6}$$

In the equations above, like in the previous section, $g_\mu$ and $g_\sigma$ are sampled as:

$$g_\mu = (2u_3 - 1)\ln(10) \tag{7}$$

$$g_\sigma = (1 - |2u_3 - 1|)\frac{\ln(10)}{3}u_4 \tag{8}$$

Here at $u_3 = 0$, $g_\mu = g_\mu^{\min} = \ln(0.1)$ and at $u_3 = 1$, $g_\mu = g_\mu^{\max} = \ln(10)$, which are the natural logarithms of the two extents of the mean aspect ratio as described in the main text. The expression for $g_\sigma$ is designed to make it approach zero whenever $u_3 = 0$ or $u_3 = 1$, and becomes its maximum value of $\frac{\ln(10)}{3}u_4$ at $u_3 = 0.5$. The magnitude of the maximum value can only be $\frac{\ln(10)}{3}$ at $u_4 = 1$, which is again 1/6th value of $g_\mu^{\max} - g_\mu^{\min}$ to keep the dispersity in aspect ratio within the $3\sigma$ limit of the normal distribution.

### S1.3. Orientational Anisotropy Parameter ($\kappa$)

Since the $\kappa$ parameter, as defined in the von Mises-Fisher distribution, can vary over a wide range from 0

[†] These authors contributed equally to this work.
[‡] Corresponding author. Email: arthij@udel.edu

(which means isotropic order) to $\infty$ (for unidirectional anisotropic order), we need to sample $\kappa$ very close to $\kappa = 0$ and $\kappa \to \infty$. To achieve this, we vary $\kappa$ over the logarithimic scale, with 25% values sampled from $\kappa = 10^{-10}$ to $\kappa = 0.1$, representing values very close to $\kappa = 0$ and another 25% from $\kappa = 10$ to $\kappa = 10^{10}$, representing values very close to $\kappa \to \infty$. The remaining 50% of the values are sampled from $\kappa = 0.1$ to $\kappa = 10$. This sampling is obtained from $u_5$ as:

$$\kappa = \begin{cases} 10^{36u_5-10} & \text{if } u_5 \leq 0.25 \\ 10^{4u_5-2} & \text{if } 0.25 < u_5 \leq 0.75 \\ 10^{36u_5-26} & \text{if } u_5 > 0.75 \end{cases} \tag{9}$$

## S2. MORE DETAILS ON SCATTERING CALCULATIONS

### S2.1. Detailed analytical form factor of a spheroid

The form factor $f_n(\mathbf{q})$ of a spheroid with $a_n$ and $c_n$ as the lengths of its semi-minor and semi-major axes, at the scattering vector $\mathbf{q} = q(\cos\theta, \sin\theta, 0)$ to calculate the scattering profile in the $xy$-plane, can be expressed as:

$$f_n(\mathbf{q}) \equiv f_n(q,\theta) = \frac{3\sin(qr_n(\theta)) - qr_n(\theta)\cos(qr_n(\theta))}{(qr_n(\theta))^3} \tag{10}$$

$$r_n(\theta) = \sqrt{a_n^2\cos^2\theta + c_n^2\sin^2\theta} \tag{11}$$

### S2.2. Finite Size Effects Correction to the Scattering Profile

As described by Brisard et al.[1], a correction scheme can be applied to the finite size effect by essentially subtracting the form factor of the cubic box from the scattering profile, after weighting it with respect to the volume fraction of all particles. This can be expressed as:

$$A_{\text{comp}}(\mathbf{q}) = \sum_{n=1}^{N} \Delta\rho_n v_n f_n(\mathbf{q}) \exp(-i\ \mathbf{q}\cdot\mathbf{r}_n) \tag{12}$$
$$- \Delta\bar{\rho} V f_{\text{box}}(\mathbf{q}) \tag{13}$$

Here $\Delta\bar{\rho}$ is the average scattering length density from all particles that is considered homogeneously over the entire cubic box, and $V = \sum_{n=1}^{N} v_n$ is the sum of the volumes of all particles. The form factor of the box $f_{\text{box}}(\mathbf{q})$ can be obtained analytically similar to $f_n(\mathbf{q})$.

## S3. HYPER-PARAMETER TUNING WITH BAYESIAN OPTIMIZATION

The hyper-parameters in XGBoost are initialized using a histogram-based algorithm, which is sped up by training on CUDA-enabled machines to leverage GPU usage and to accelerate computations. Over fitting is reduced by using regularization terms such as lamda and alpha, penalizing overly complex models, controlling depth and complexity of individual decision trees using pruning, are among the many possible options that can be tuned to improve the training of the XGBoost model. To compute the loss during training, we used negative mean squared error:

**Table** S1. **Bayesian Search Optimization of Hyper-parameters.**

| Hyper-parameter | Search Range | Optimum Value |
|---|---|---|
| column sample by tree | 0.5 – 1.0 | 0.899 |
| column sample by level | 0.5 – 1 | 0.799 |
| gamma | 0 – 1 | 0.6 |
| learning rate | 0.001 – 0.1 | 0.082 |
| maximum depth | 3 – 15 | 14 |
| minimum child weight | 1 – 10 | 6 |
| n estimators | 50 – 1000 | 200 |
| lambda | 0.1 – 1 | 0.9 |
| alpha | 0.1 – 1 | 0.70 |
| sub-sample | 0.5 – 1 | 0.799 |

$$L = -\frac{1}{n}\sum_{i=1}^{n}(y_i - \hat{y}_i)^2$$

With such a variety of hyper-parameters we conducted Bayesian search optimization by first defining a parameter space and then finding optimum values within this space as shown in **Table S1**. Here we used 50 iterations and employed a 5-fold cross-validation scheme which uses Gaussian process regression. Each hyper parameter has a specific role in defining the architecture of the complete XGBoost decision tree as elaborated below:

1. *column sample by tree* determines the fraction of features randomly sampled to build each tree
2. *column sample by level* determines the fraction of features randomly sampled at each level
3. *gamma* controls node splitting based on the expected reduction in loss
4. *learning rate* dictates the step size in each iteration
5. *maximum depth* limits the maximum depth of a tree to prevent over-fitting
6. *minimum child weight* sets the minimum sum of weights required in a child node
7. *n estimators* sets number of boosting rounds or trees used
8. *lambda* parameter that controls L2 regularization
9. *alpha* parameter that controls L1 regularization

10. *sub-sample* determines the fraction of observations randomly sampled for building each tree

## S4. VALIDATION OF THE SURROGATE ML MODEL

For the four test samples shown in **Figure 4** of the main text, with Sample IDs 1076, 1097, 2176 and 1910, the original and predicted intensity values are compared as overlayed 1D profiles of $I(q,\theta)$ vs $q$ at $\theta = 0°, 60°$ and $120°$ in Figure S1.

## S5. MORE DETAILS AND VALIDATION OF GENETIC ALGORITHM OPTIMIZATION IN CREASE-2D

### S5.1. Normalization of Structural Features to Genes

Similar to the random sampling scheme for structural features, as described in section S1, an analoguous scheme to describe 6 normalized genes $g_1, g_2, ...g_6$ that correspond to $R_\mu$, $R_\sigma$, $\gamma_\mu$, $\gamma_\sigma$, $\kappa$ and $\phi$ can be described as shown below:

$$g_1 = \frac{r_\mu - \ln(3)}{\ln(10)} \tag{14}$$

$$g_2 = \frac{6r_\sigma}{\ln(10)(1 - |2g_1 - 1|)} \tag{15}$$

$$g_3 = \frac{g_\mu - \ln(3)}{\ln(10)} \tag{16}$$

$$g_4 = \frac{3g_\sigma}{\ln(10)(1 - |2g_3 - 1|)} \tag{17}$$

$$g_5 = \begin{cases} \frac{1}{36}\left(\log\left(\kappa\right) + 10\right) & \text{if } \kappa \leq 0.1 \\ \frac{1}{4}\left(\log\left(\kappa\right) + 2\right) & \text{if } 0.1 < \kappa \leq 10 \\ \frac{1}{36}\left(\log\left(\kappa\right) + 26\right) & \text{if } \kappa > 10 \end{cases} \tag{18}$$

$$g_6 = 2\phi \tag{19}$$

Here, $r_\mu$,$r_\sigma$,$g_\mu$ and $g_\sigma$ were already defined with respect to $R_\mu$, $R_\sigma$, $\gamma_\mu$, $\gamma_\sigma$ in section S1.

### S5.2. Validation of the GA Optimization Loop

For the four test samples that were shown in **Figure 4** of the main text, with Sample IDs 1076, 1097, 2176 and 1910, we compare the fitness of their independent GA runs for 1000 generations in **Figure S2**. In **Figure S3**, the remaining 2 plots for Sample IDs 1097 and 2176 are shown.

## REFERENCES

[1] S. Brisard and P. Levitz, Small-angle scattering of dense, polydisperse granular porous media: Computation free of size effects, Physical Review E **87**, 013305 (2013).

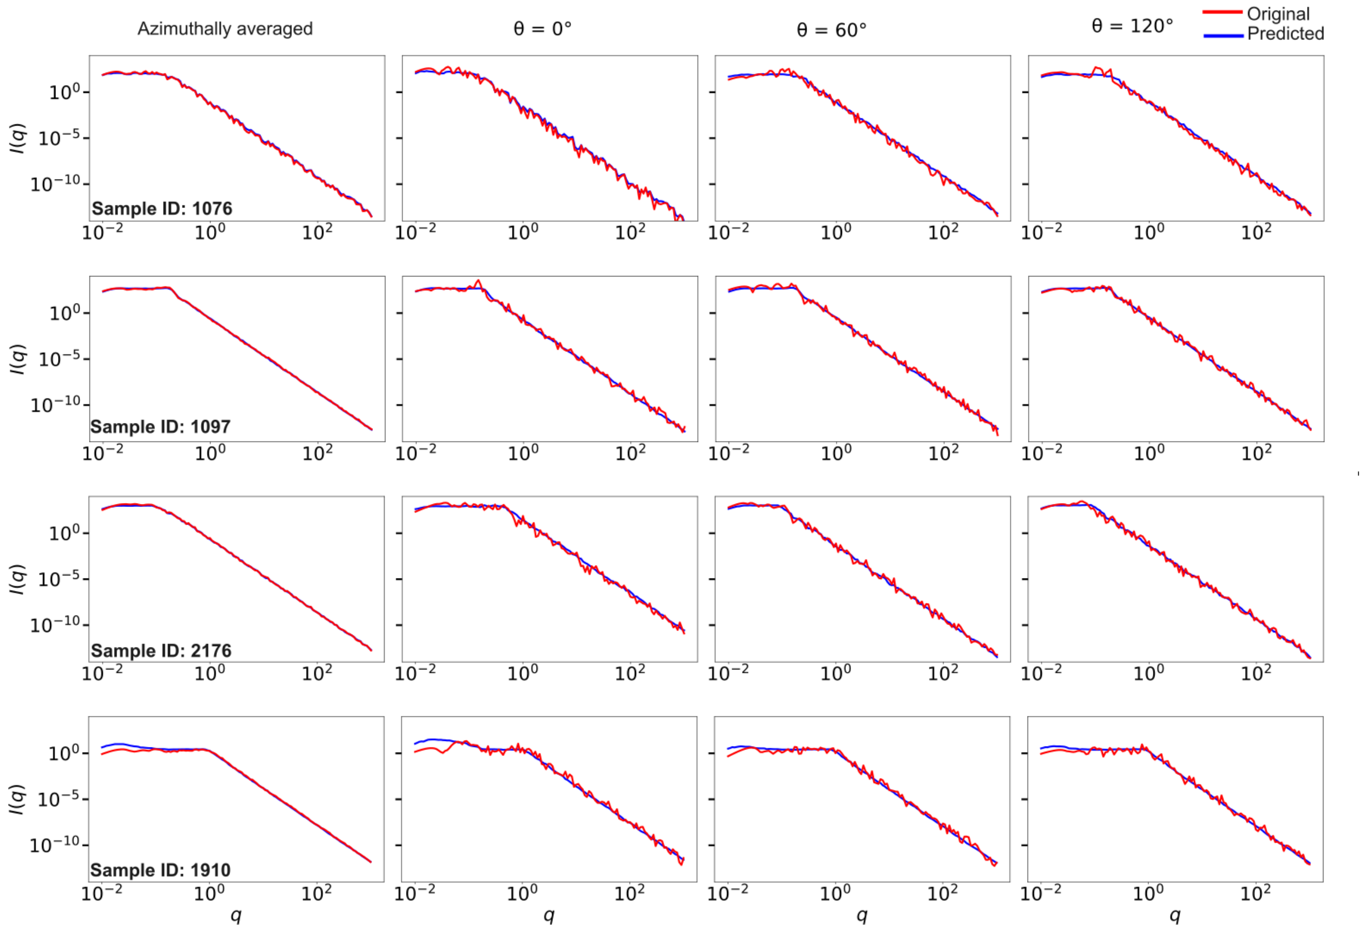


**Fig.** S1. Comparison of 1D scattering profiles from ML predictions and original 1D scattering profiles, azimuthally averaged as well as at specific $\theta valuesasdenotedabove$

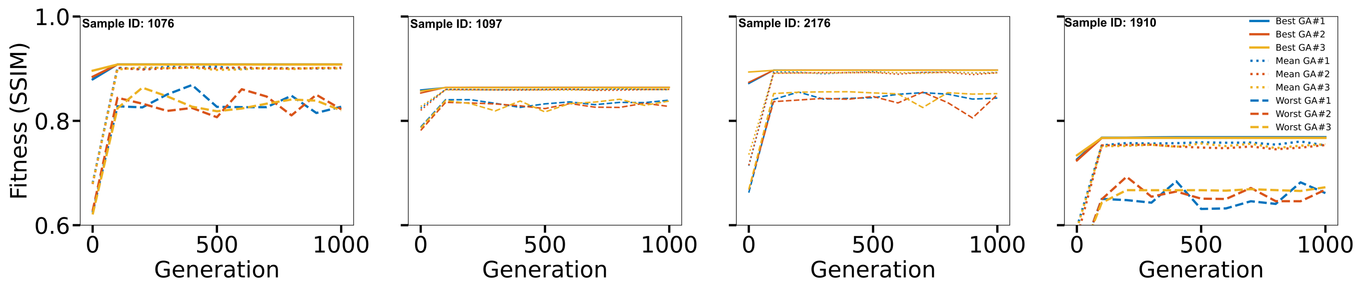


**Fig.** S2. Plots of fitness evolution over a 1000 generations for 3 GA runs for Sample IDs 1076, 1097, 2176 and 1910. Legend shows the evolution of the individuals with the best, mean, and worst fitness in each generation

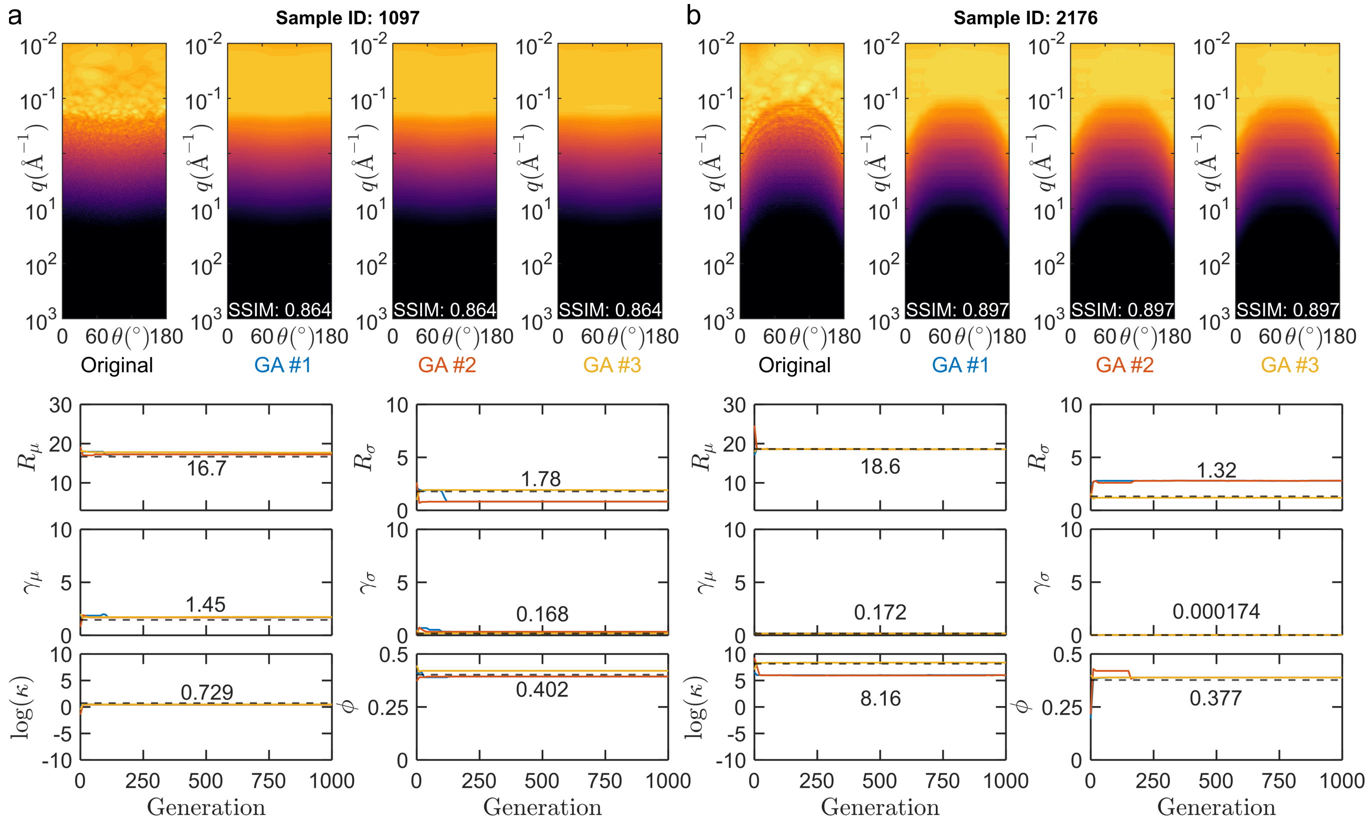


**Fig.** S3. Performance of Genetic Algorithm (GA) in CREASE-2D.(a-b) Two other samples - Sample IDs 1097 and 2176- out of the 600 samples tested with CREASE-2D. We show visual comparison of the input scattering profile and outputs from three independent GA runs and plot their corresponding evolution of structural feature predictions during each GA run for Sample IDs 1097 and 2176. Like the main paper, the three colored lines in the plots are the three GA runs' evolution of that structural feature; black dashed and text shows the original profile's value for that structural feature
